# Supplementary material for: Enhancing Incomplete Multi-modal Brain Tumor Segmentation with Intra-modal Asymmetry and Inter-modal Dependency
Source: arXiv:2406.10175 source file (2024-06-14)
Supplement: Supplementary file 1 [file Additional_peer_comparison.tex]

\begin{figure*}[ht]
  \centering
    \includegraphics[width=0.99\linewidth]{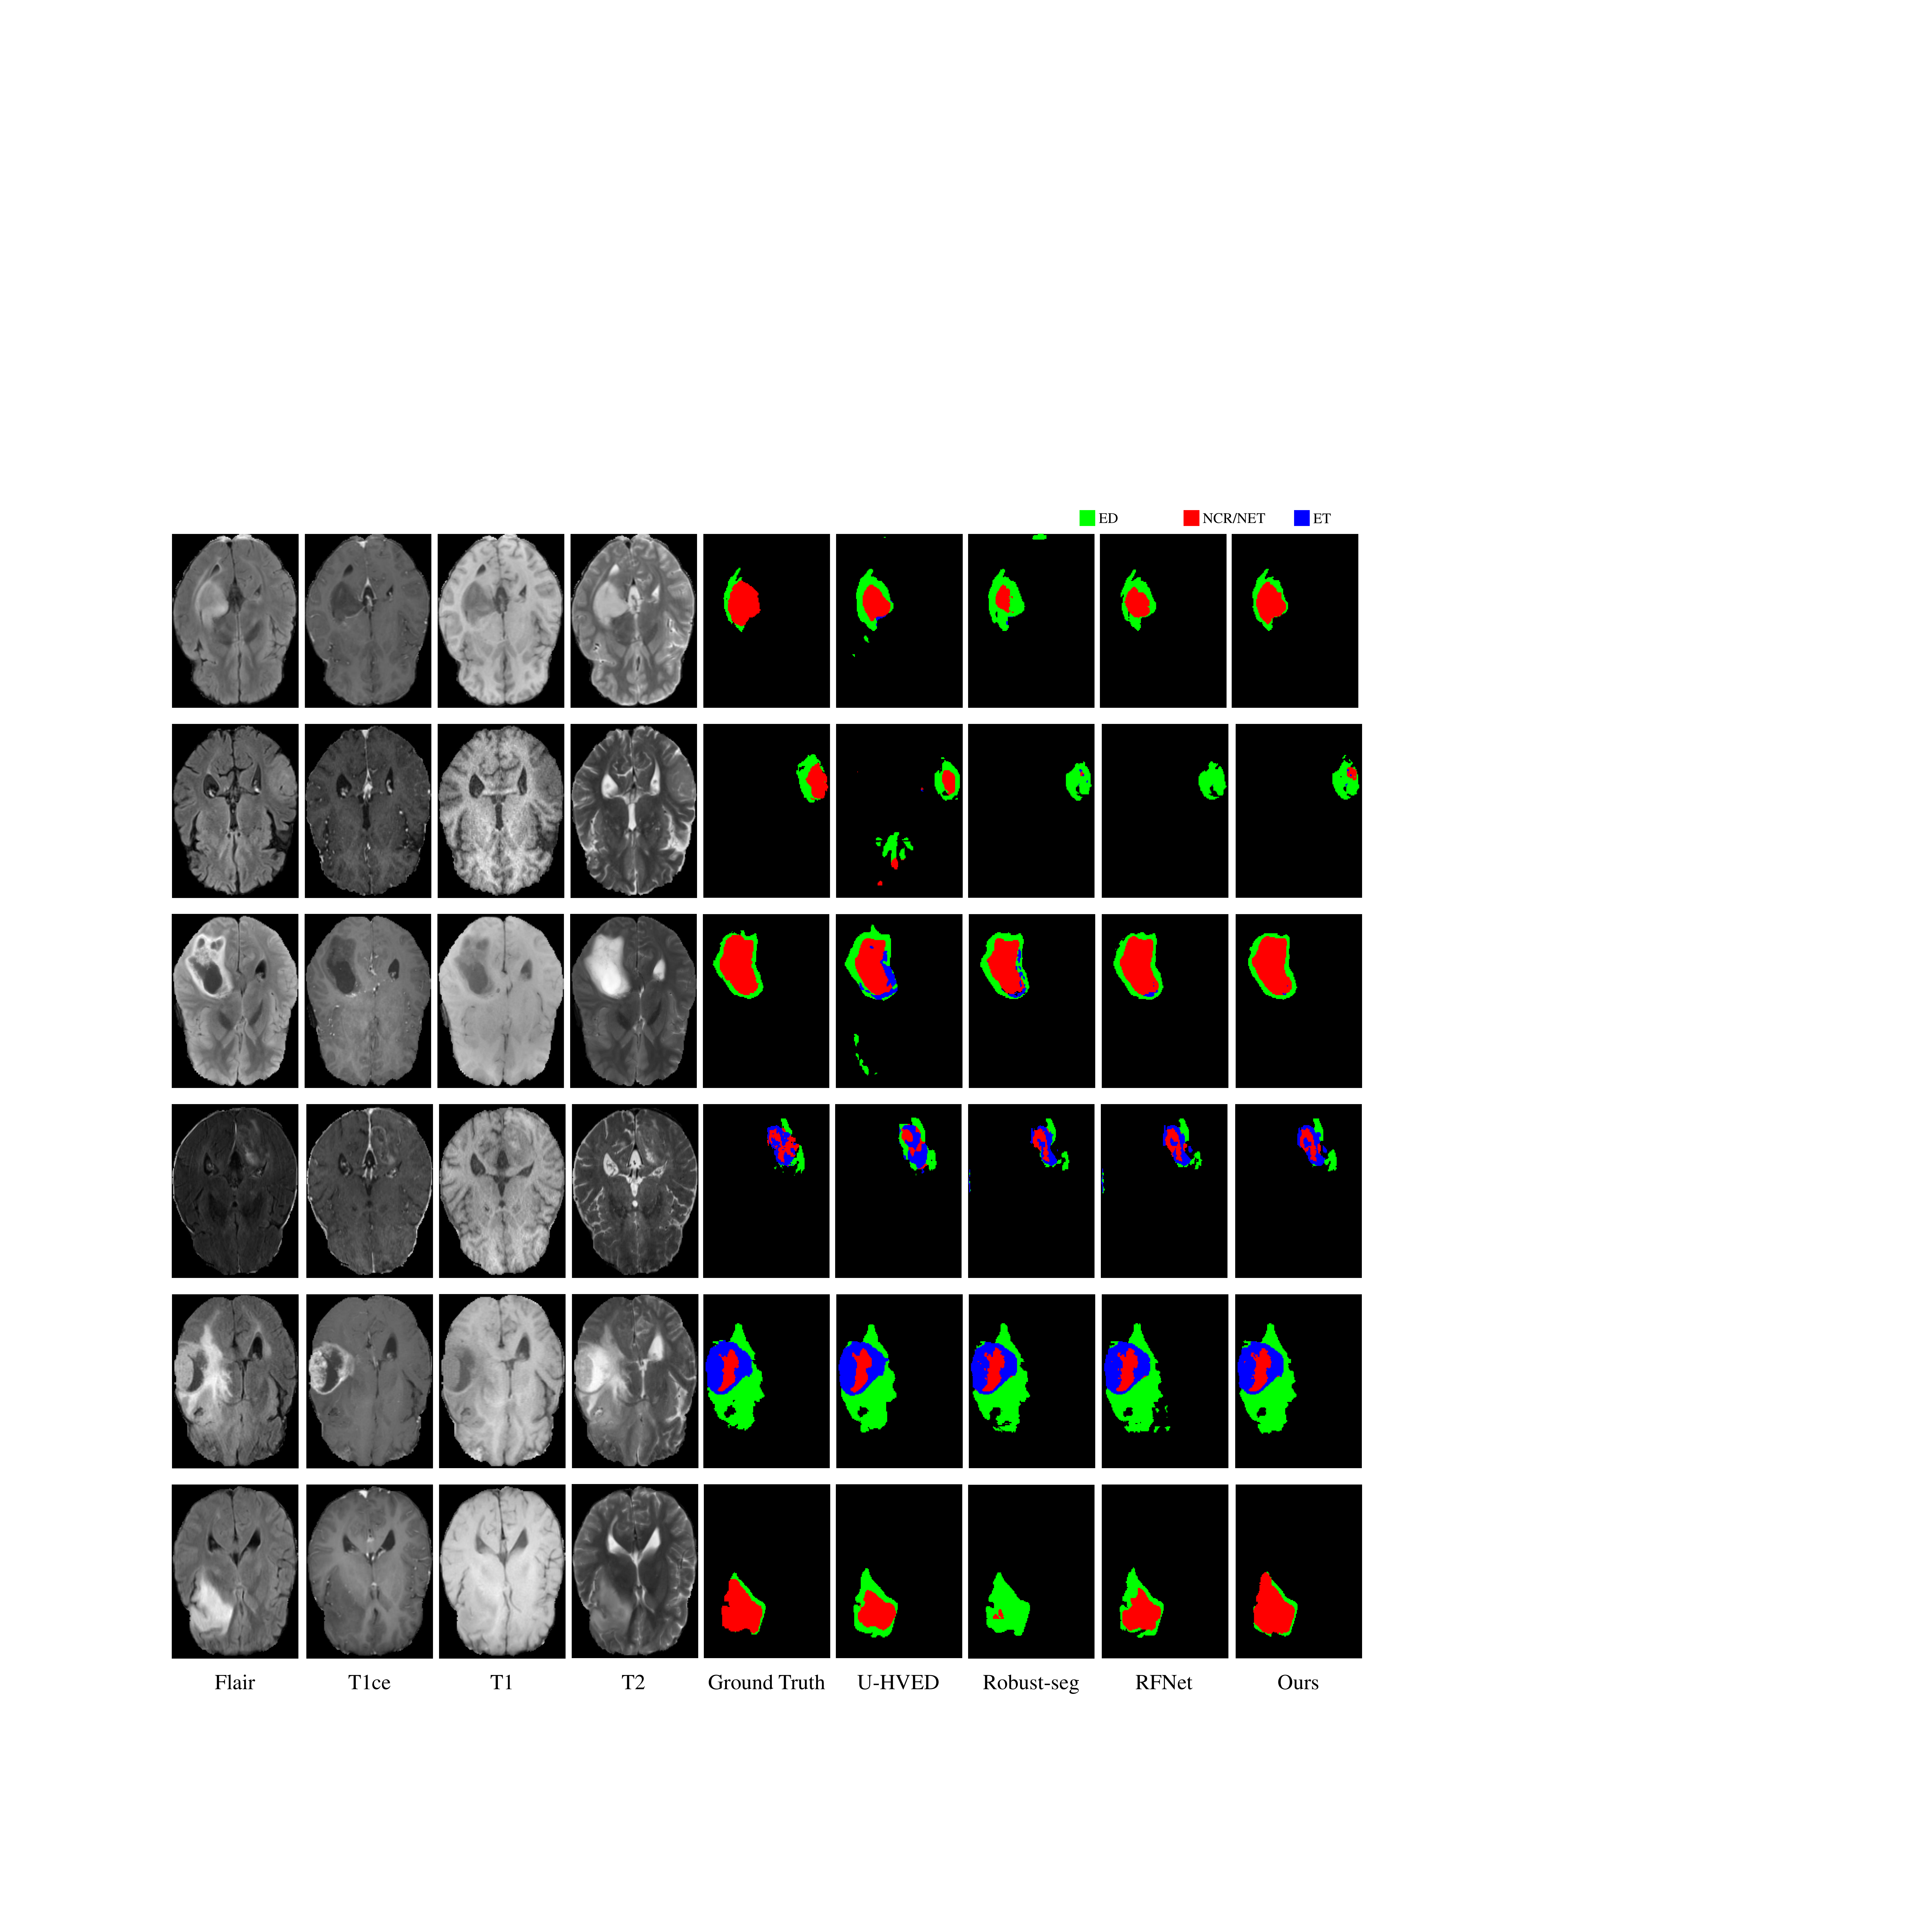}
    \caption{Additional visualization of segmentation results between our method and state-of-the-art methods. From left to right, we demonstrate the MRI images for Flair modality, T1ce modality, T1 modality and T2 modality. Following the ground truth, the prediction of U-HVED\cite{dorent2019hetero}, RobustSeg\cite{chen2019robust}, RFNet\cite{ding2021rfnet} and our prediction. 
    }
    \label{Figure: Additional_peer_comparison}
\end{figure*}
