# Supplementary material for: Enhancing Incomplete Multi-modal Brain Tumor Segmentation with Intra-modal Asymmetry and Inter-modal Dependency
Source: arXiv:2406.10175 source file (2024-06-14)
Supplement: Supplementary file 2 [file Additional_post-training.tex]

\begin{figure*}[ht]
  \centering
    \includegraphics[width=0.7\linewidth]{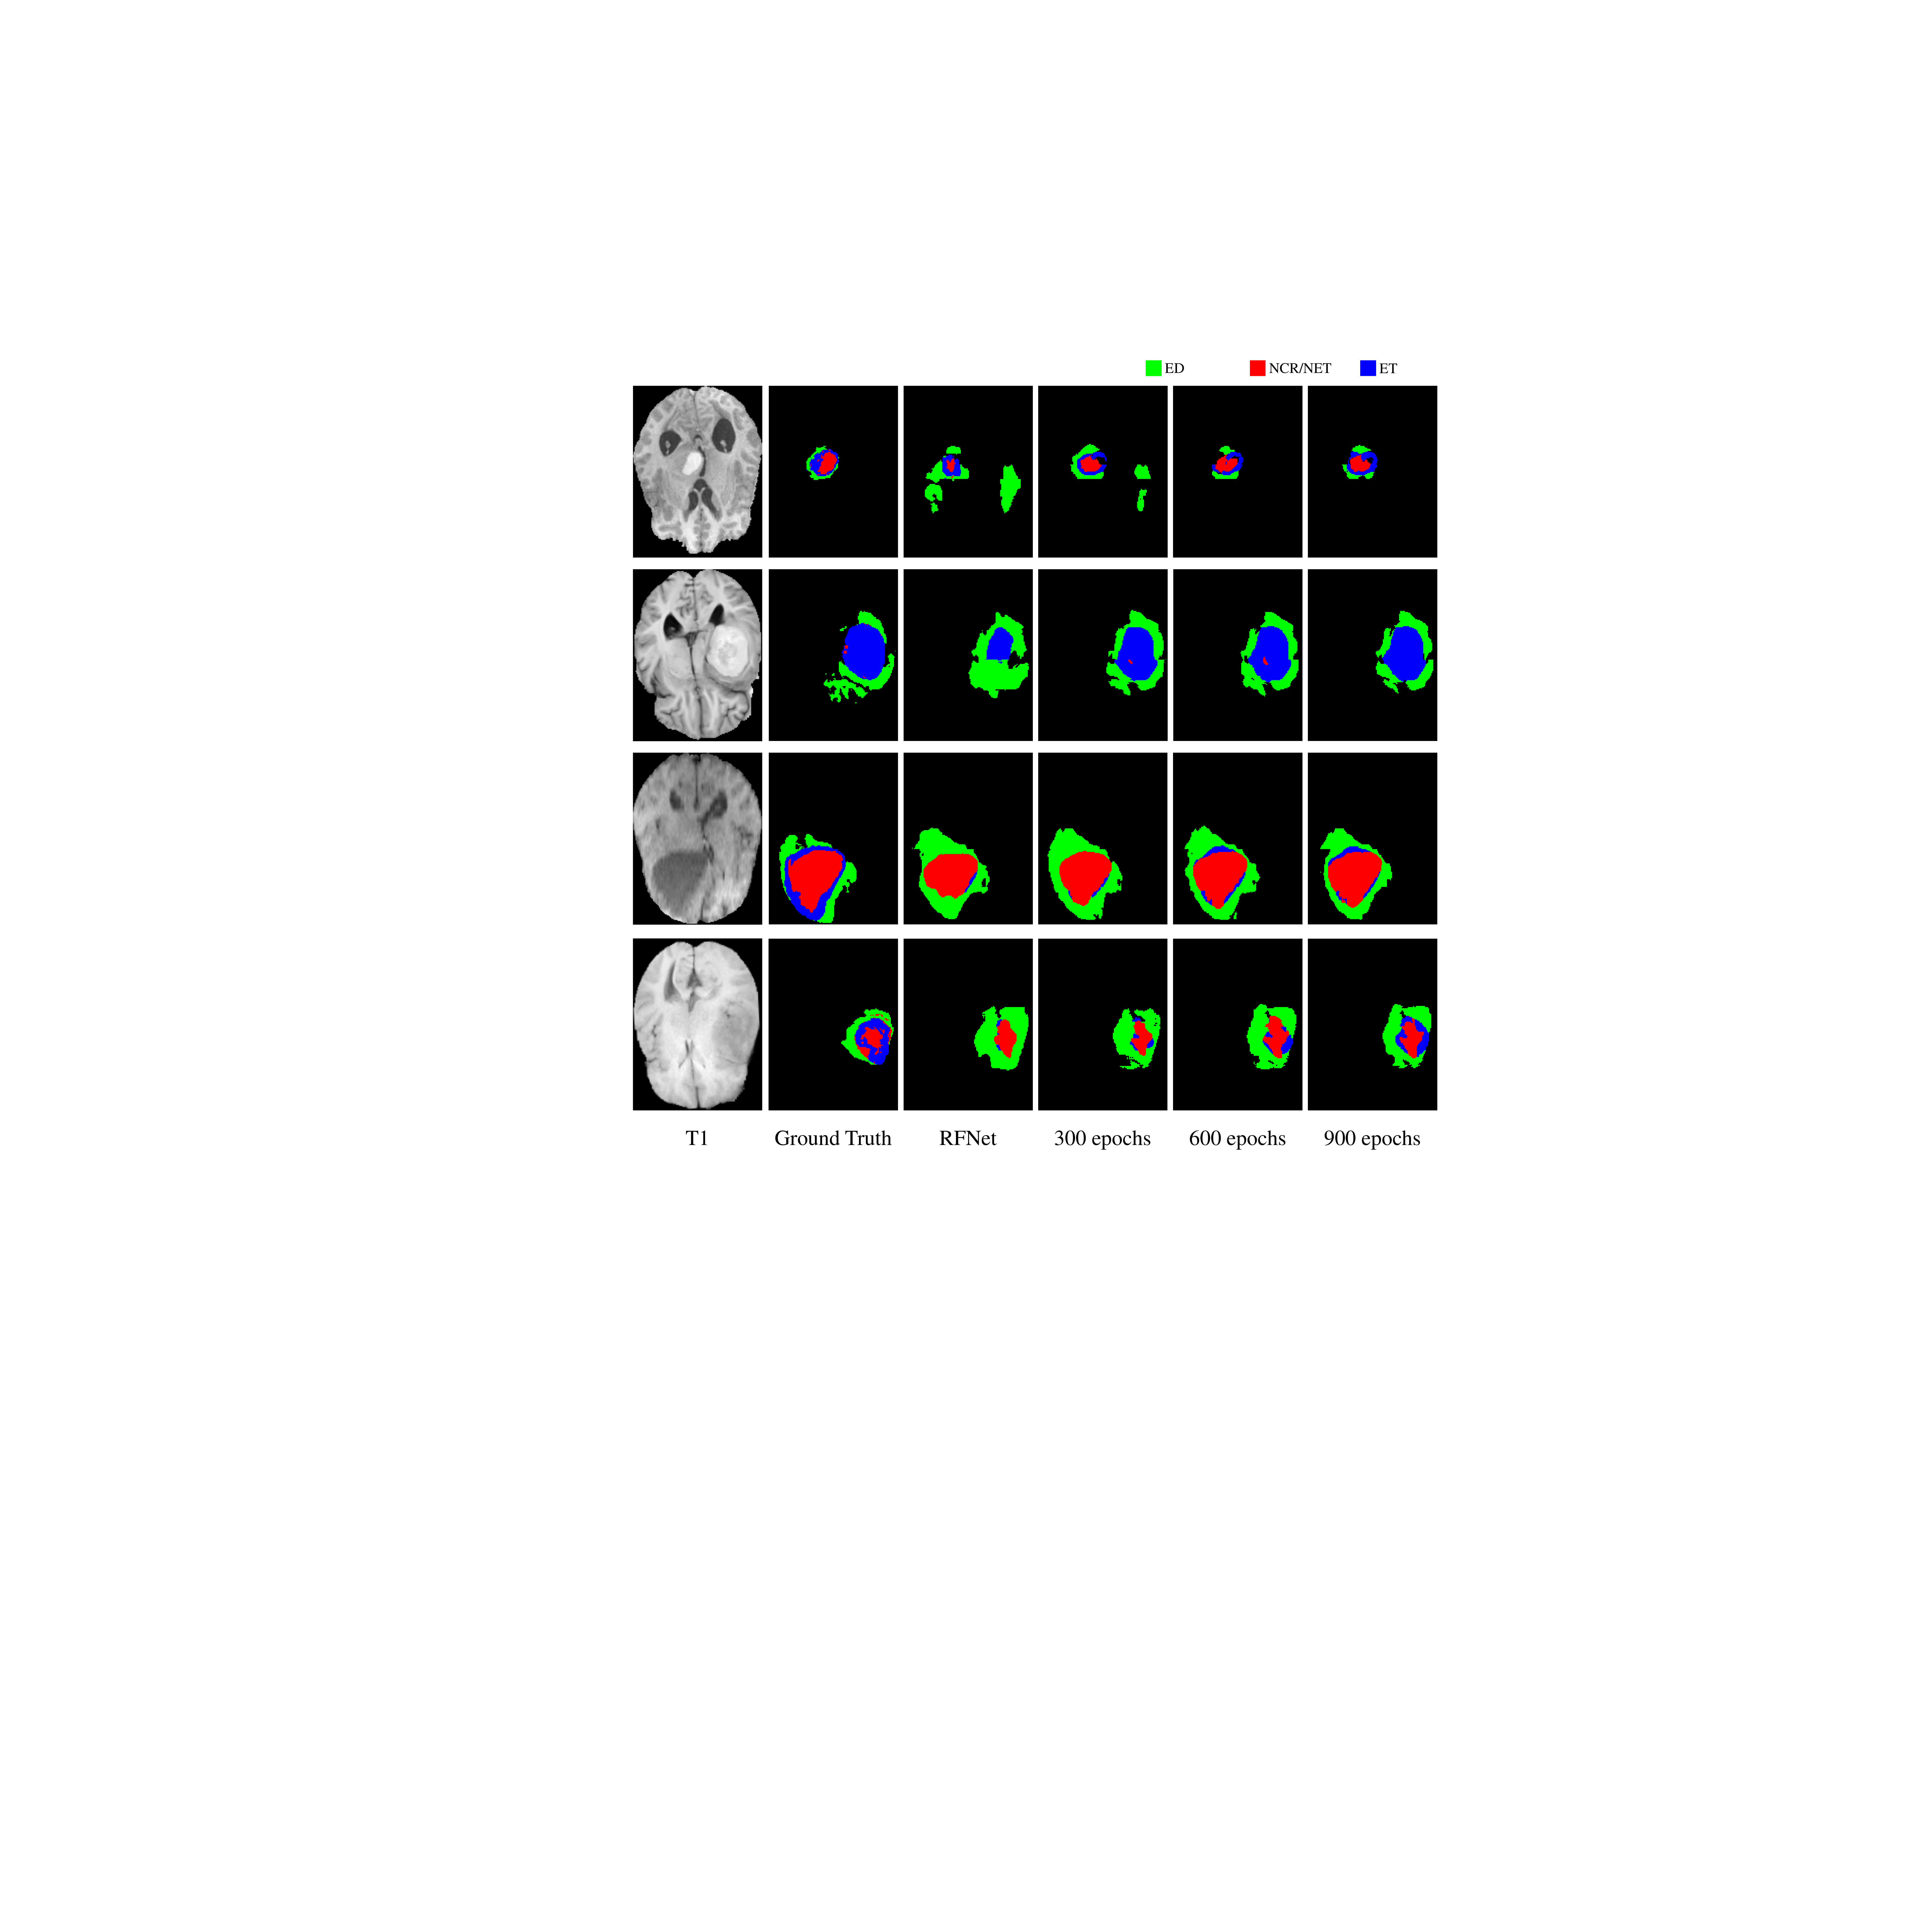}
    \caption{Additional visualization of the prediction of different iterations for the KD-based post-training, while only T1 modality is input into the networks for prediction.}
    \label{Figure: Additional_post-training}
\end{figure*}
